# Supplementary material for: Charge coloration dynamics of electrochromic amorphous tungsten oxide studied by simultaneous electrochemical and color impedance measurements
Source: arXiv:2011.03895 ancillary file (2020-11-23)
Supplement: Supplementary file 1 [file supplementary_information.pdf]

Supplementary Information

# Charge coloration dynamics of electrochromic amorphous tungsten oxide studied by simultaneous electrochemical and color impedance measurements

Edgar A. Rojas-González[1, a)] and Gunnar A. Niklasson[1]
*Department of Materials Science and Engineering, The Ångström Laboratory, Uppsala University, P.O. Box 35, SE-751 03 Uppsala, Sweden*

(Dated: 23 November 2020)

[a)]Electronic mail: edgar.rojas@angstrom.uu.se.

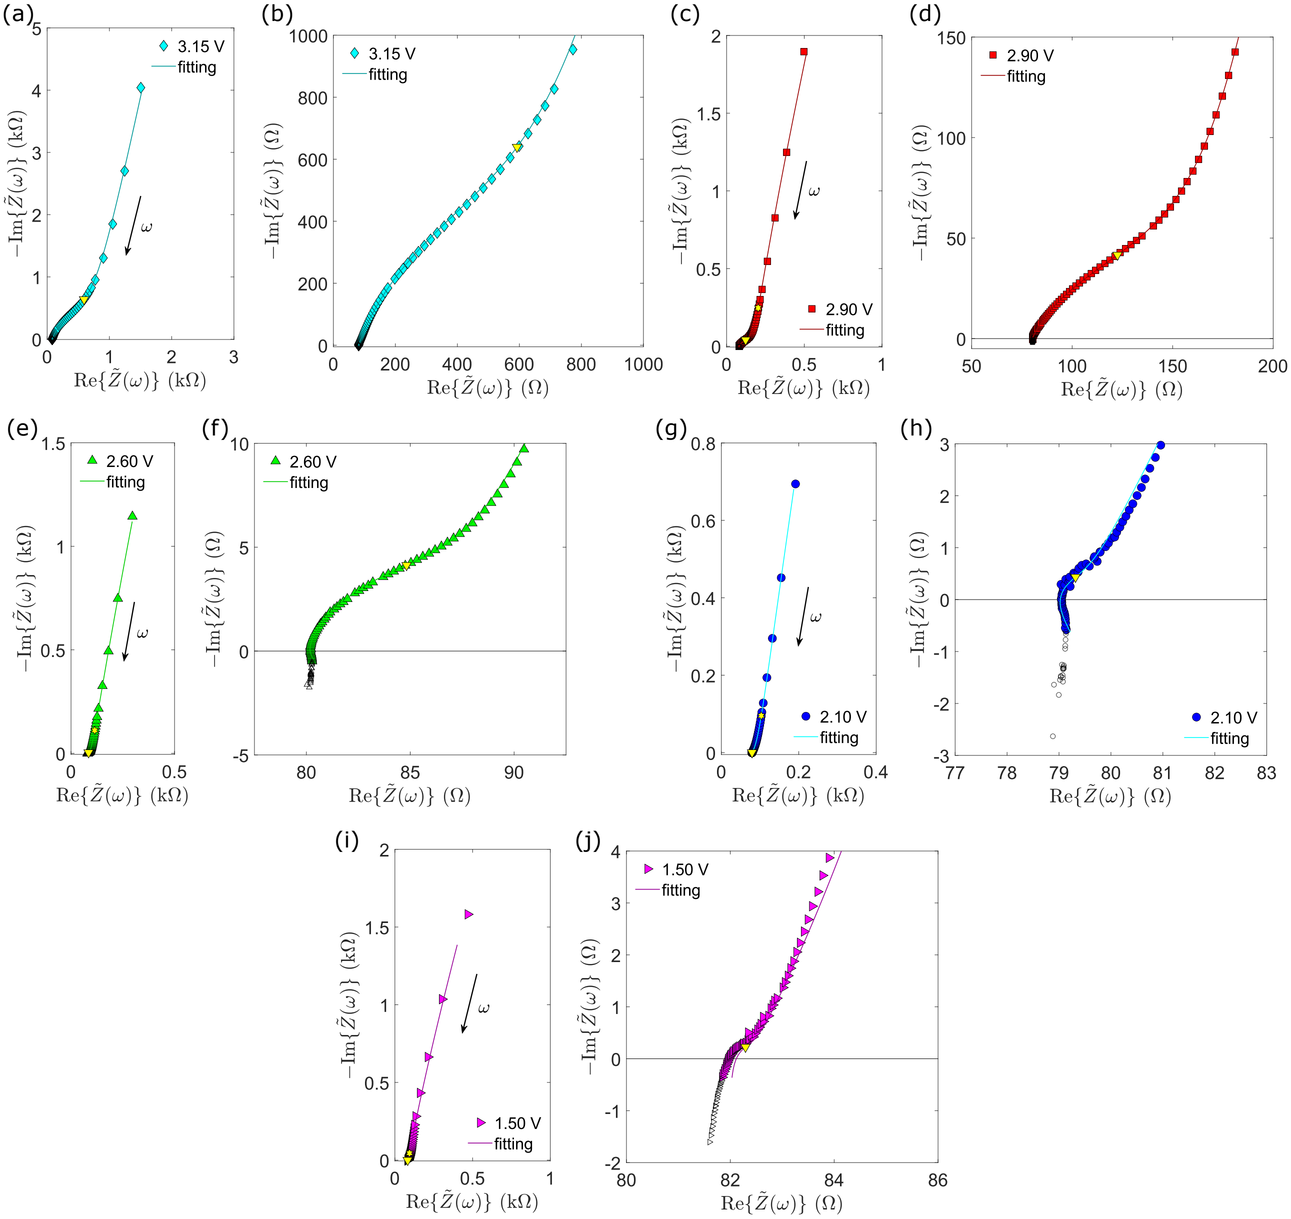


FIG. S1. Nyquist plots of the EIS spectra for the $a\mathrm{WO_3}$ film measured at the equilibrium bias potentials, with respect to $\mathrm{Li/Li^+}$, of 3.15 V (a), 2.90 V (c), 2.60 V (e), 2.10 V (g), and 1.50 V (i). The arrows point toward the direction of increasing frequency $\omega$. Panels (b), (d), (f), (h), and (j) display respectively an expanded view of the high-frequency region of the data depicted in (a), (c), (e), (g), and (i). The filled symbols represent the experimental data, and the solid lines correspond to the fittings to the equivalent circuit presented in Fig. 1(b) in the main text—both are displayed in the frequency range of 10 mHz-10 kHz. The small unfilled symbols portray the experimental data in the high-frequency range of 10 kHz-30 kHz. The points of the fitting lines evaluated at the linear frequencies $f_\mathrm{D} = \omega_\mathrm{D}/2\pi$ (yellow stars)—characteristic linear frequency of diffusion—and $f_\mathrm{ad} = \omega_\mathrm{ad}/2\pi$ (yellow downward-facing triangles)—characteristic linear frequency of the adsorption process—are indicated in the plots. $\omega_\mathrm{D}$ and $\omega_\mathrm{ad}$ are defined in the main text in Eqs. (7) and (14), respectively.

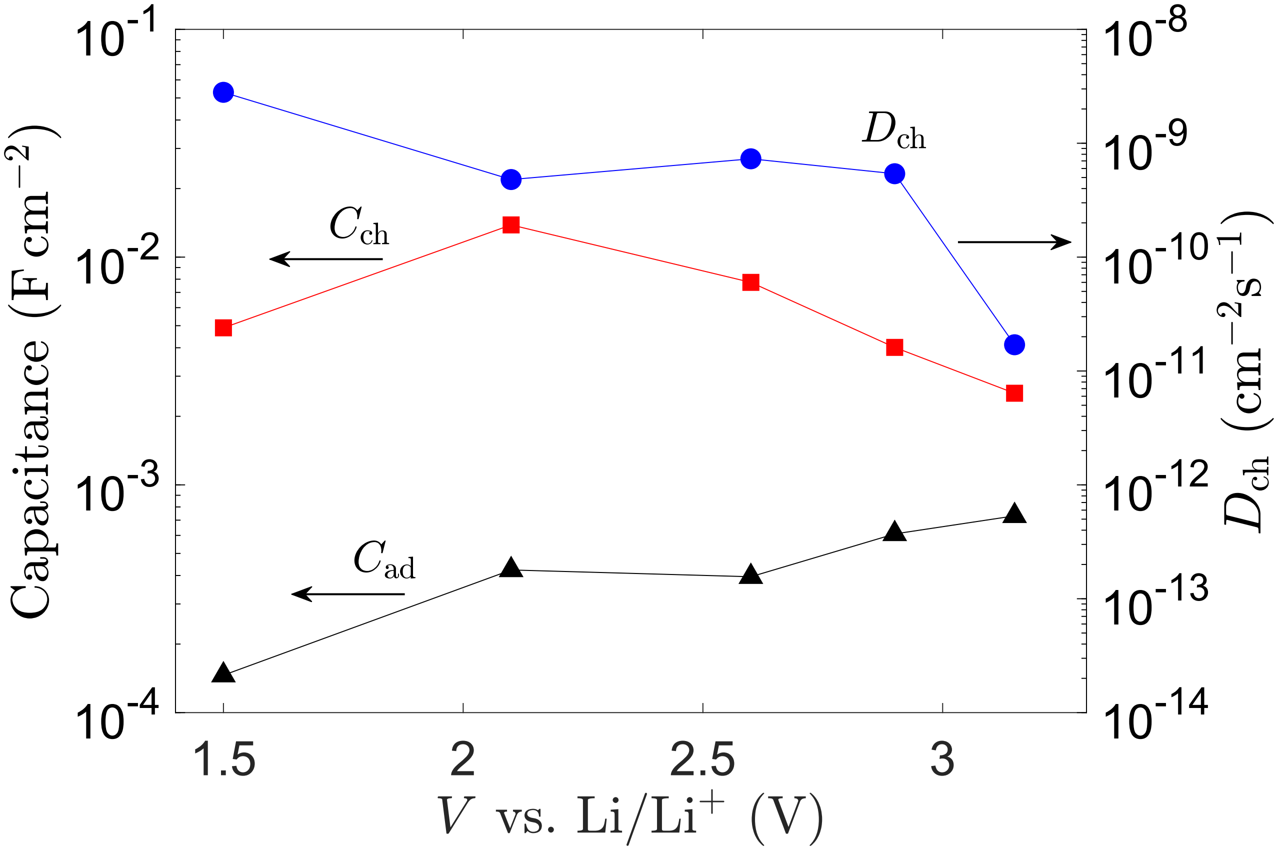


FIG. S2. Effective adsorption $C_{ad}$ and chemical $C_{ch}$ capacitances (per unit area) as well as chemical diffusion coefficient $D_{ch}$ as a function of equilibrium bias potential for the $a$WO$_3$ film.

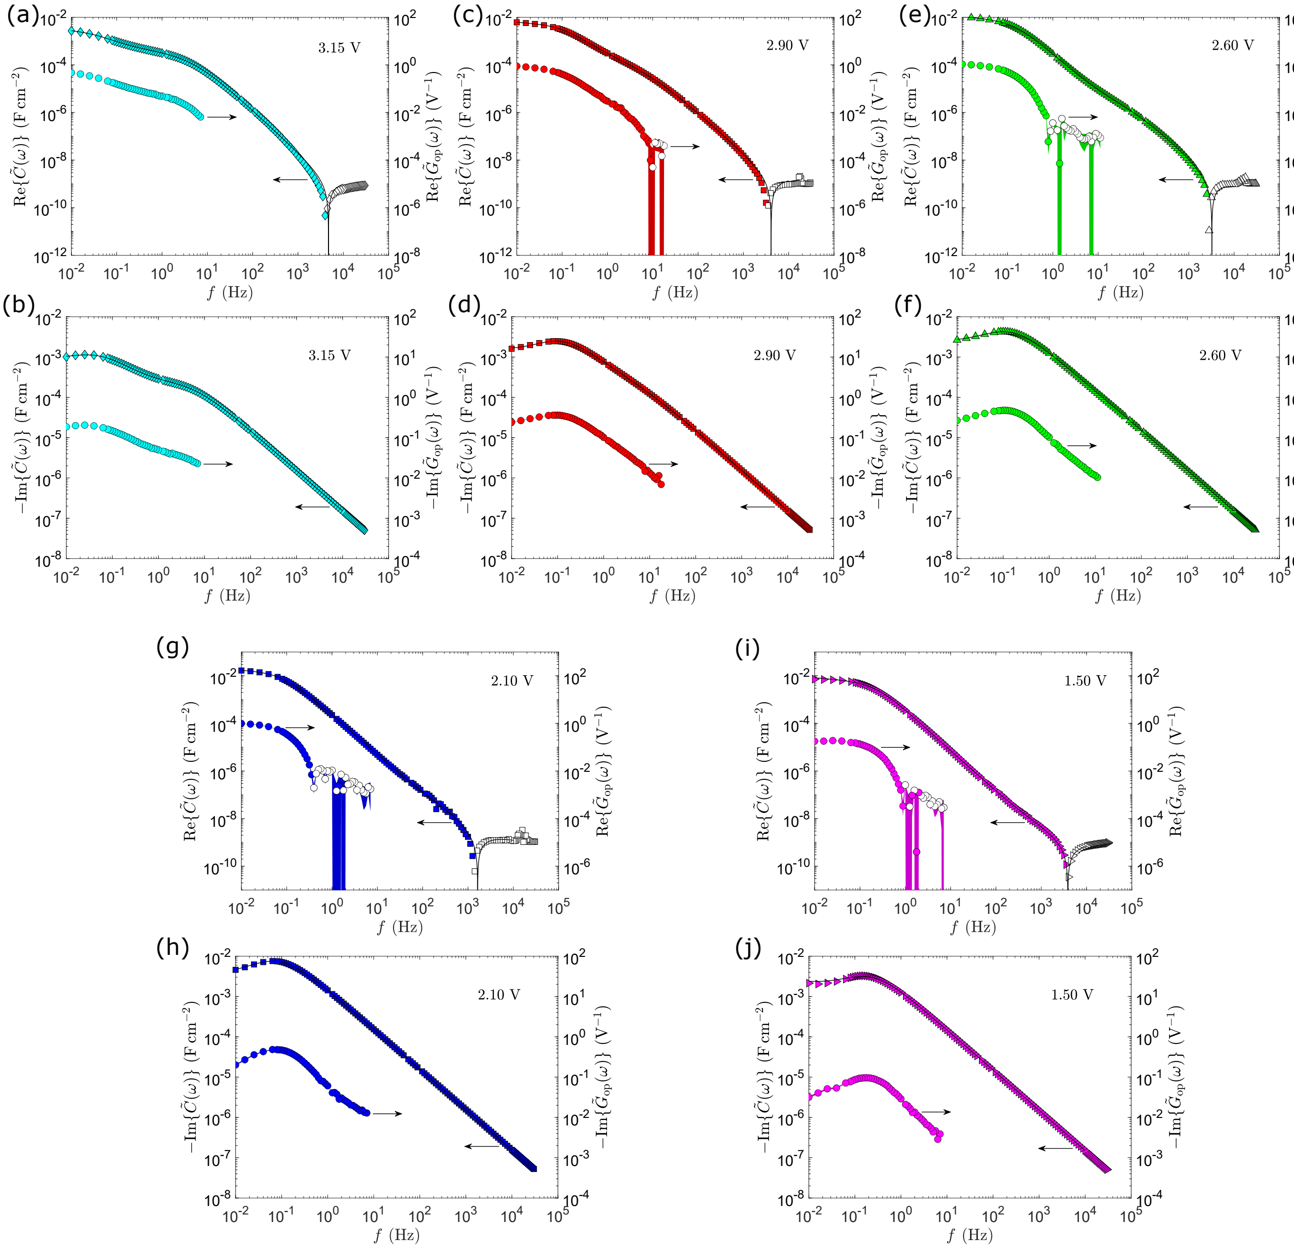


FIG. S3. Bode plots of the real—(a), (c), (e), (g), and (i)—and imaginary—(b), (d), (f), (h), and (j)—parts of the complex capacitance $\tilde{C}(\omega)$ and complex optical capacitance $\tilde{G}_{\mathrm{op}}(\omega)$ for the $a\mathrm{WO}_3$ film measured at the equilibrium bias potentials, with respect to $\mathrm{Li}/\mathrm{Li}^+$, given in each plot. The $\tilde{C}(\omega)$ data are displayed in the frequency range of 10 mHz-30 kHz. In this case, the fittings to the equivalent circuit presented in Fig. 1(b) are portrayed by solid black lines for frequencies between 10 mHz and 10 kHz. $\tilde{C}(\omega)$ and $\tilde{G}_{\mathrm{op}}(\omega)$ are defined in Eqs. (4) and (5) in the main text, respectively. In panels (a), (c), (e), (g), and (i), the unfilled symbols correspond to data values with $\mathrm{Re}\{\tilde{C}(\omega)\} < 0$ and $\mathrm{Re}\{\tilde{G}_{\mathrm{op}}(\omega)\} < 0$. The shaded regions around the $\tilde{G}_{\mathrm{op}}(\omega)$ curves depict one standard deviation with respect to the experimental values.
